# Supplementary material for: A Domain Specific Language for Testing Consensus Implementations
Source: arXiv:2303.05893 source file (2023-04-22)
Supplement: Supplementary file 1 [file appendix.tex]

\section{Appendix for Section~\ref{system_model}}
\label{appendix:system_model}

Complete proof of Theorem~\ref{thm:main}.

We define a prefix relation $\preceq$ between two histories $H_1 = (E_1, <_1)$ and $H_2 = (E_2, <_2)$. We say, $H_1 \preceq H_2$ if 
\begin{enumerate}
    \item Downward closure: $E_1 \subseteq E_2$ and for some event $e\in E_2$. If $e \in E_1$, then $\forall e', e' <_2 e \Rightarrow e' \in E_1 \land e' <_1 e$.
    \item Happens before preservation: For two events $e, e' \in E_1$, $e <_1 e' \Leftrightarrow e <_2 e'$
\end{enumerate}

\setcounter{theorem}{0}
\begin{theorem}
    For any complete run $\rho$ in the protocol $\protocol$, there exists a monitor $\monitor$ such that, for all executions $\rho'$ in the product transition system of $\protocol$ and $\monitor$. $H_{\rho'} \preceq H_{\rho}$
\end{theorem}
\begin{proof}
    For the given execution $\rho$ and history $H = H_{\rho} = (E_{\rho}, <_{\rho})$, we define $O_H: M_\rho \rightarrow 2^{E_\rho}$, a function that maps a message $m$ to events $e'$ that \textit{happen before} the receive event $e = (m.to, receive, m)$.  ($M_{\rho}$ is the set of all messages received by replicas in the execution $\rho$)
    \[O_H(m) = \left\{e \mid e <_{\rho} (m.to, receive, m)\right\}\] 
    To capture messages introduced using the \textsc{Adversary} rule, we define $Adv_H$
    \[Adv_H = \left\{m \mid (m.to, receive, m) \in E_{\rho} \land (m.from, send, m) \notin E_{\rho}\right\}\] 
    
    We now define the monitor $\mu$. The states of the monitor are $s \in \monitorStates = (pool, E)$ where $pool \subseteq \allMessages$ is the set of pending messages and $E \subseteq \allEvents$ is the set of events that have already occurred. The initial state is $\monitorInit = (\phi,\phi)$. We define the transition function of the monitor as $\monitorTransition(s,e) = (s', M)$, where

    \begin{align*}
        s'.E =&\; s.E \cup \left\{e\right\} \\
        M =& \left\{m \mid m \in (p' \cup Adv_H) \land m \in M_{\rho} \land O_H(m) \subseteq s'.E\right\} \\
        s'.pool =&
        \begin{cases}
            (s.pool \cup \left\{m\right\}) \setminus M & \mbox{if } e = (m.from, send, m) \\
            s.pool \setminus M & \mbox{otherwise} \\
        \end{cases}
    \end{align*}
    and $p' = \begin{cases}
        (s.pool \cup \left\{m\right\}) & \mbox{if } e = (m.from, send, m) \\
        s.pool & \mbox{otherwise} \\
    \end{cases}$

    Consider any execution in the product transition system $\rho' = C_0 \xrightarrow{l_0} C_1 \xrightarrow{l_1} \cdots \xrightarrow{l_{g-1}} C_g$. 
    We first prove that $H_{\rho'} \preceq H_{\rho}$. 
    
    First we prove the downward closure property. For any event $e \in E_{\rho}$, 
    \[e \in E_{\rho'} \Rightarrow (\forall e', e'<_{\rho}e \Rightarrow e' \in E_{\rho'} \land e' <_{\rho'} e)\]

    Let us consider the case when $e = (m.to, receive, m)$. We know that in $\rho'$ every \textsc{Receive} step at $i$ is preceded by a \textsc{Monitor} step at $j < i$. That is, $\monitorTransition(s_j,e_j) = (s_{j+1}, M)$ where $m \in M$. By the definition of $M$, 
    \begin{enumerate}
        \item $O_H(m) \subseteq s_{j+1}.E \subseteq E_{\rho'}$. In other words all events $e'$ where $e' <_\rho e$ we can say that $e' \in E_{\rho'}$. Furthermore, we can say that $e'$ has occurred in $\rho'$ at step $j < i$. When $e'$ is in the same replica, by the definition of \textit{happens before}, this is sufficient to say that $e' <_{\rho'} e$.
        \item $m \in M_{\rho}$. This implies that $M_{\rho'} \subseteq M_{\rho}$
    \end{enumerate}

    As a consequence of (1), let $(e_1, e_2, \cdots, e_k)$ be the sequence of receive events at a replica $r \in \allReplicas$ in the execution $\rho$. Consider the largest $i$ such that $e_i \in E_{\rho'}$, then we can say that $(e_1, e_2, \cdots, e_i)$ is the sequence of receive events for replica $r$ in the execution $\rho'$. In other words, the sequence of messages delivered to a replica in $\rho'$ is a prefix of the same sequence in $\rho$.

    Given a replica $r$, let $s_i$ denote the state of the replica at step $i$ in the execution $\rho$. By induction on $i$, we prove that $s_i$ is the state of the replica $r$ in the execution $\rho'$. When $i=0$, this is trivially true since the initial state is the same for both the executions. Assuming it is true at step $i$, we need to prove that $s_{i+1}$ is the state in $\rho'$. Either
    \begin{enumerate}
        \item $\protocolTransition(s_i,\bot) = (s_{i+1}, e_{i+1})$. Then, it is the same in $\rho'$ (due to the restriction on $\protocolTransition$)
        \item $\protocolTransition(s_i, m) = (s_{i+1}, e_{i+1})$. Since, the sequence of messages delivered in $\rho'$ is the same, $m$ will be the same and hence $s_{i+1}$ will also be the same.
    \end{enumerate}
    We can then say that if $(e_1, e_2, \cdots, e_k)$ is the sequence of events observed for a replica $r$ in $\rho$ and consider the largest $i$ such that $e_i \in E_{\rho'}$, then a $(e_1, e_2, \cdots, e_i)$ is the sequence of events observed for the same replica in $\rho'$.

    We now show that for any two events $e_1, e_2 \in E_{\rho}$ such that $e_1 <_{\rho} e_2$, if $e_2 \in E_{\rho'}$ then $e_1 \in E_{\rho} \land e_1 <_{\rho'} e_2$. Either, 
    \begin{enumerate}
        \item $e_1, e_2$ are in the same replica, then $(\cdots, e_1, \cdots, e_2, \cdots)$ is the sequence of events in the replica. We know that the prefix $(\cdots, e_1, \cdots, e_2)$ occurs in $\rho'$ for the same replica. Hence $e_1 \in E_{\rho'}$ and $e_1 <_{\rho'} e_2$
        \item $e_1, e_2$ are in different replicas, then $\exists e_s, e_r \in E_{\rho}$ such that $e_1 < e_s < e_r < e_2$. Furthermore, $e_1, e_s$ are in the same replica and $e_r, e_2$ are in the same replica. We know that $e_r \in E_{\rho'}$ (events in the same replica) and $e_1, e_s \in E_{\rho'}$ (events before a receive). And due to the definition of \textit{happens before}, $e_s <_{\rho'} e_r$. Using case (1), we know that $e_1 <_{\rho'} e_s$ and $e_r <_{\rho'} e_2$.
    \end{enumerate}

    To prove that happens before is preserved. It suffices to show that, for any two events $e_1, e_2 \in E_{\rho'}, e_1 <_{\rho'} e_2 \Rightarrow e_1 <_{\rho} e_2$. We use the same case analysis. Either,
    \begin{enumerate}
        \item $e_1, e_2$ are in the same replica, then $(\cdots, e_1, \cdots, e_2, \cdots)$ is the sequence of events in the replica. We know that the sequence of events for the replica in $\rho'$ is $(\cdots, e_1, \cdots, e_2, \cdots)$. Hence $e_1 \in E_{\rho'}$ and $e_1 <_{\rho'} e_2$
        \item $e_1, e_2$ are in different replicas, then $\exists e_s, e_r \in E_{\rho'}$ such that $e_1 < e_s < e_r < e_2$. Furthermore, $e_1, e_s$ are in the same replica and $e_r, e_2$ are in the same replica. And due to the definition of \textit{happens before}, $e_s <_{\rho} e_r$. Using case (1), we know that $e_1 <_{\rho} e_s$ and $e_r <_{\rho} e_2$.
    \end{enumerate}
\end{proof}
